# Supplementary material for: Simple few-shot method for spectrally resolving the wavefront of an ultrashort laser pulse
Source: arXiv:2307.15799 source file (2024-02-26)

**(a)**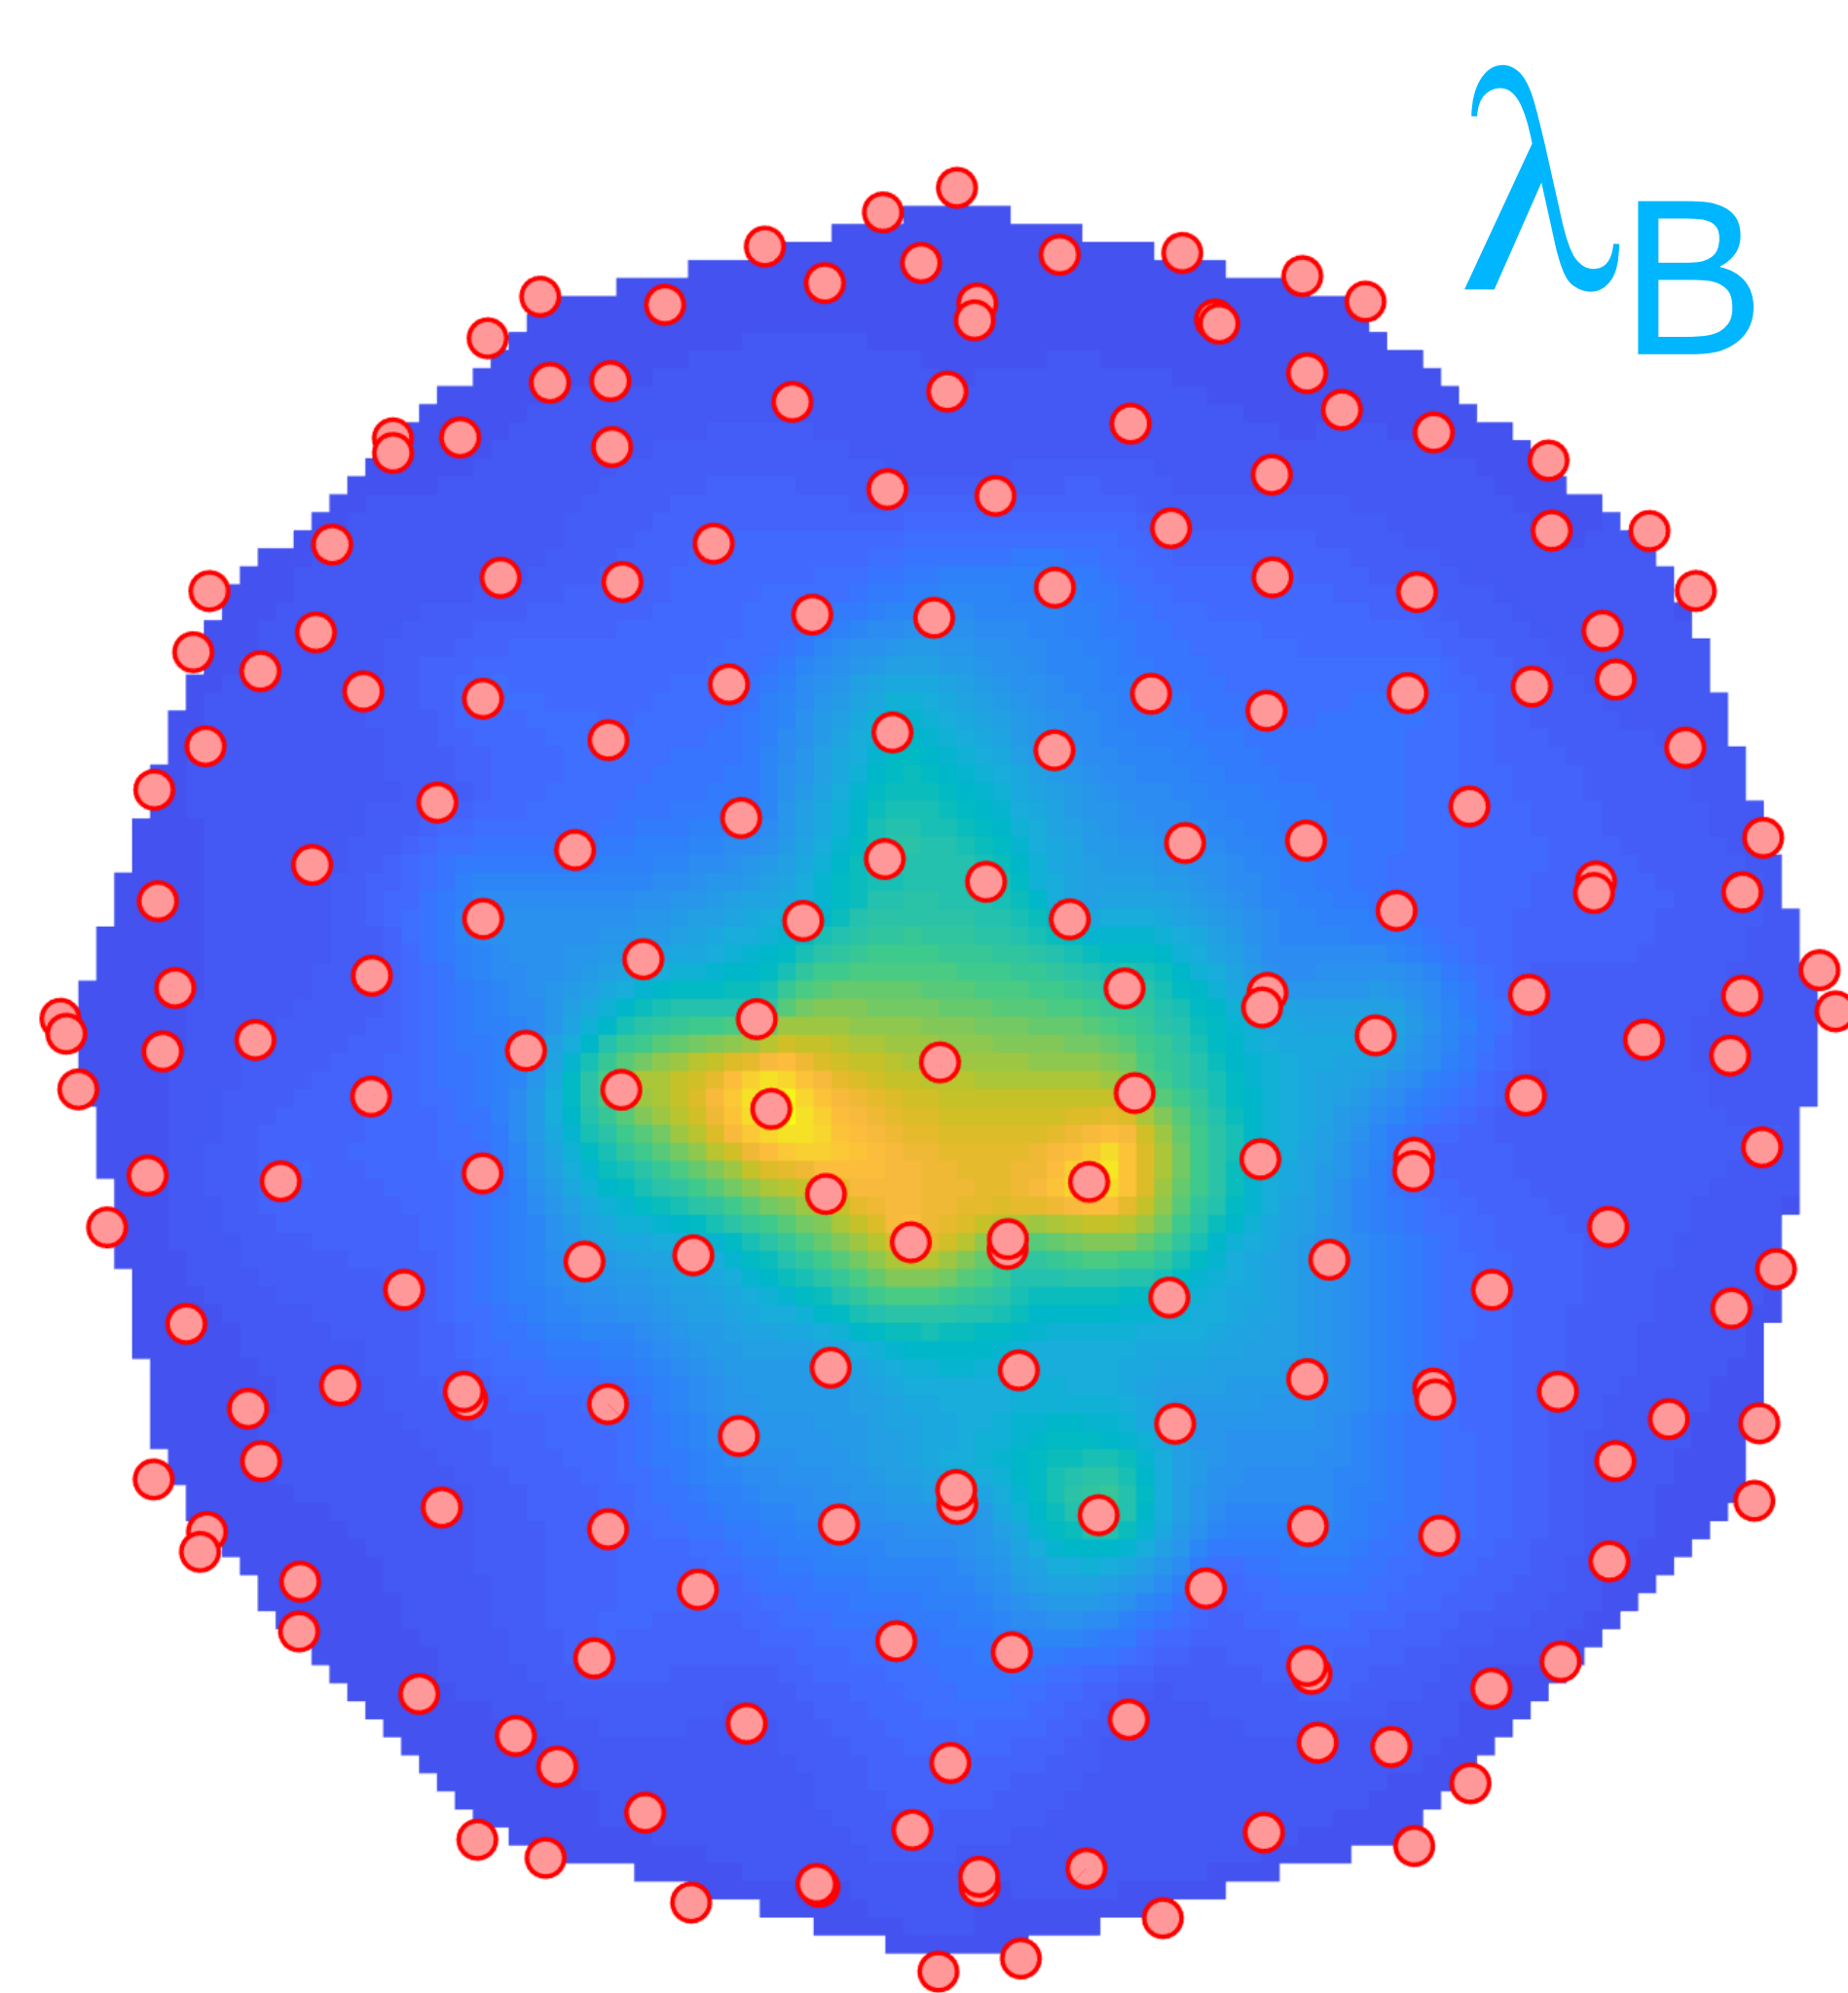**(b)**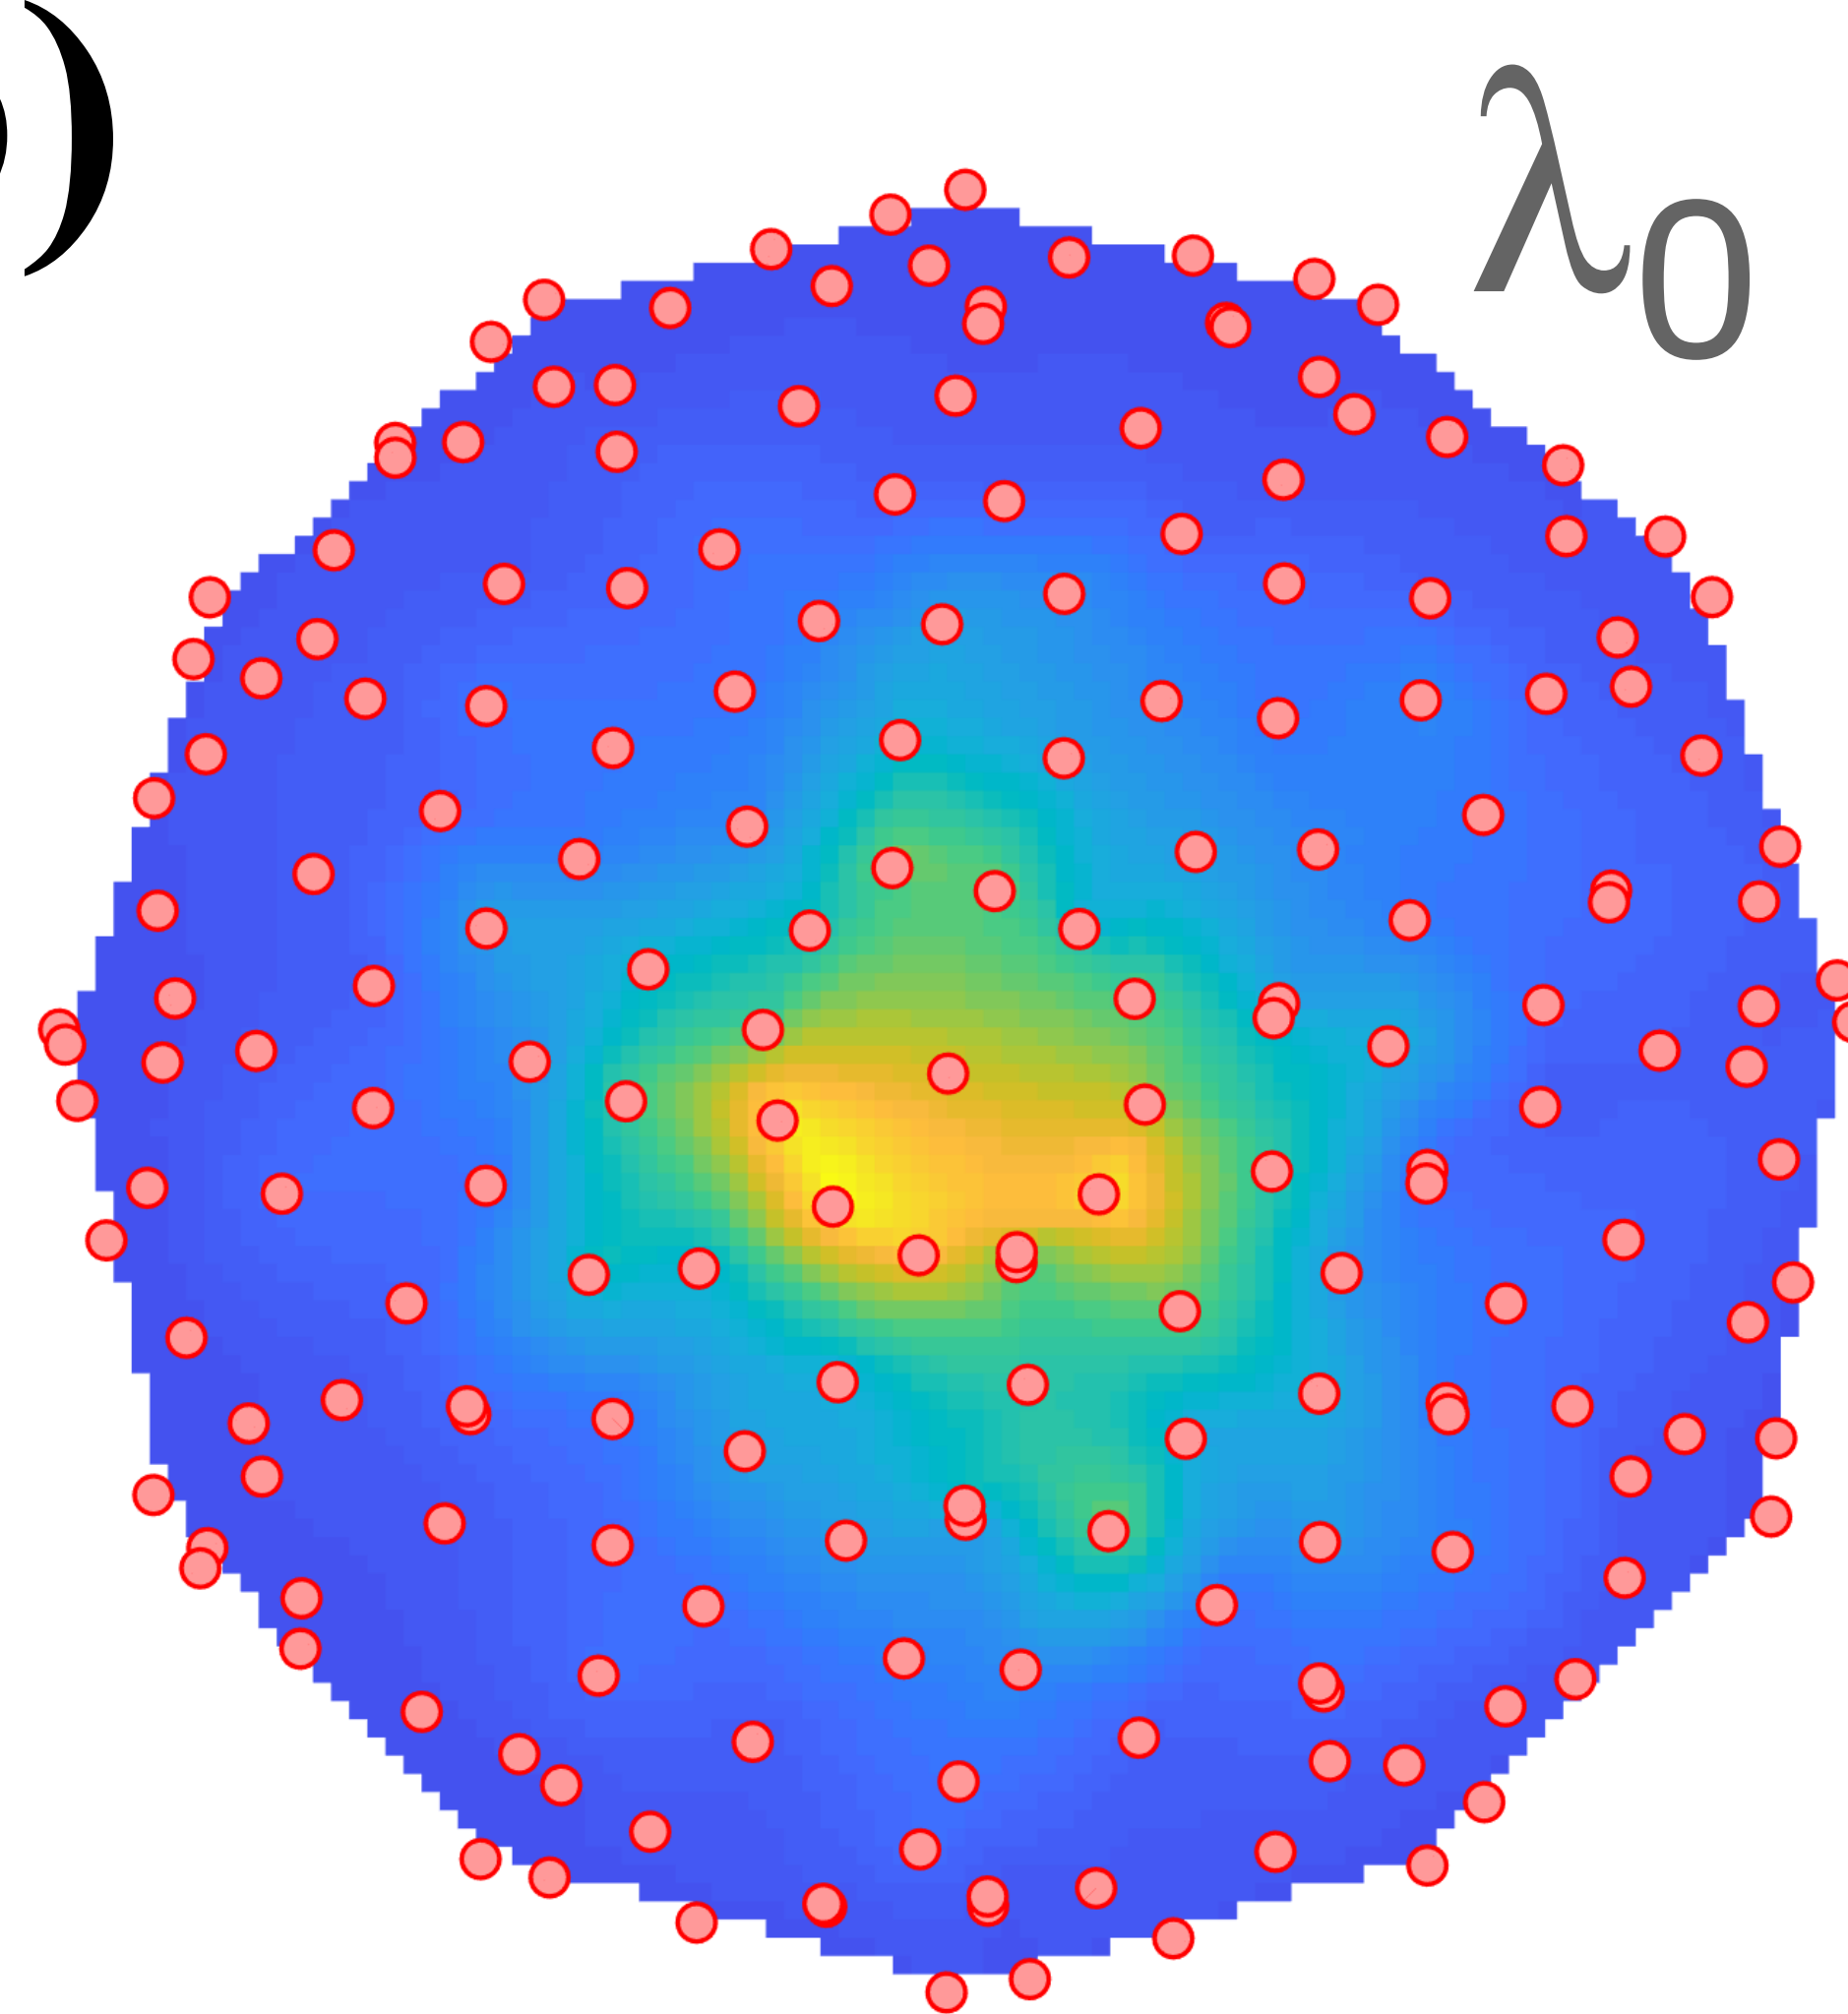**(c)**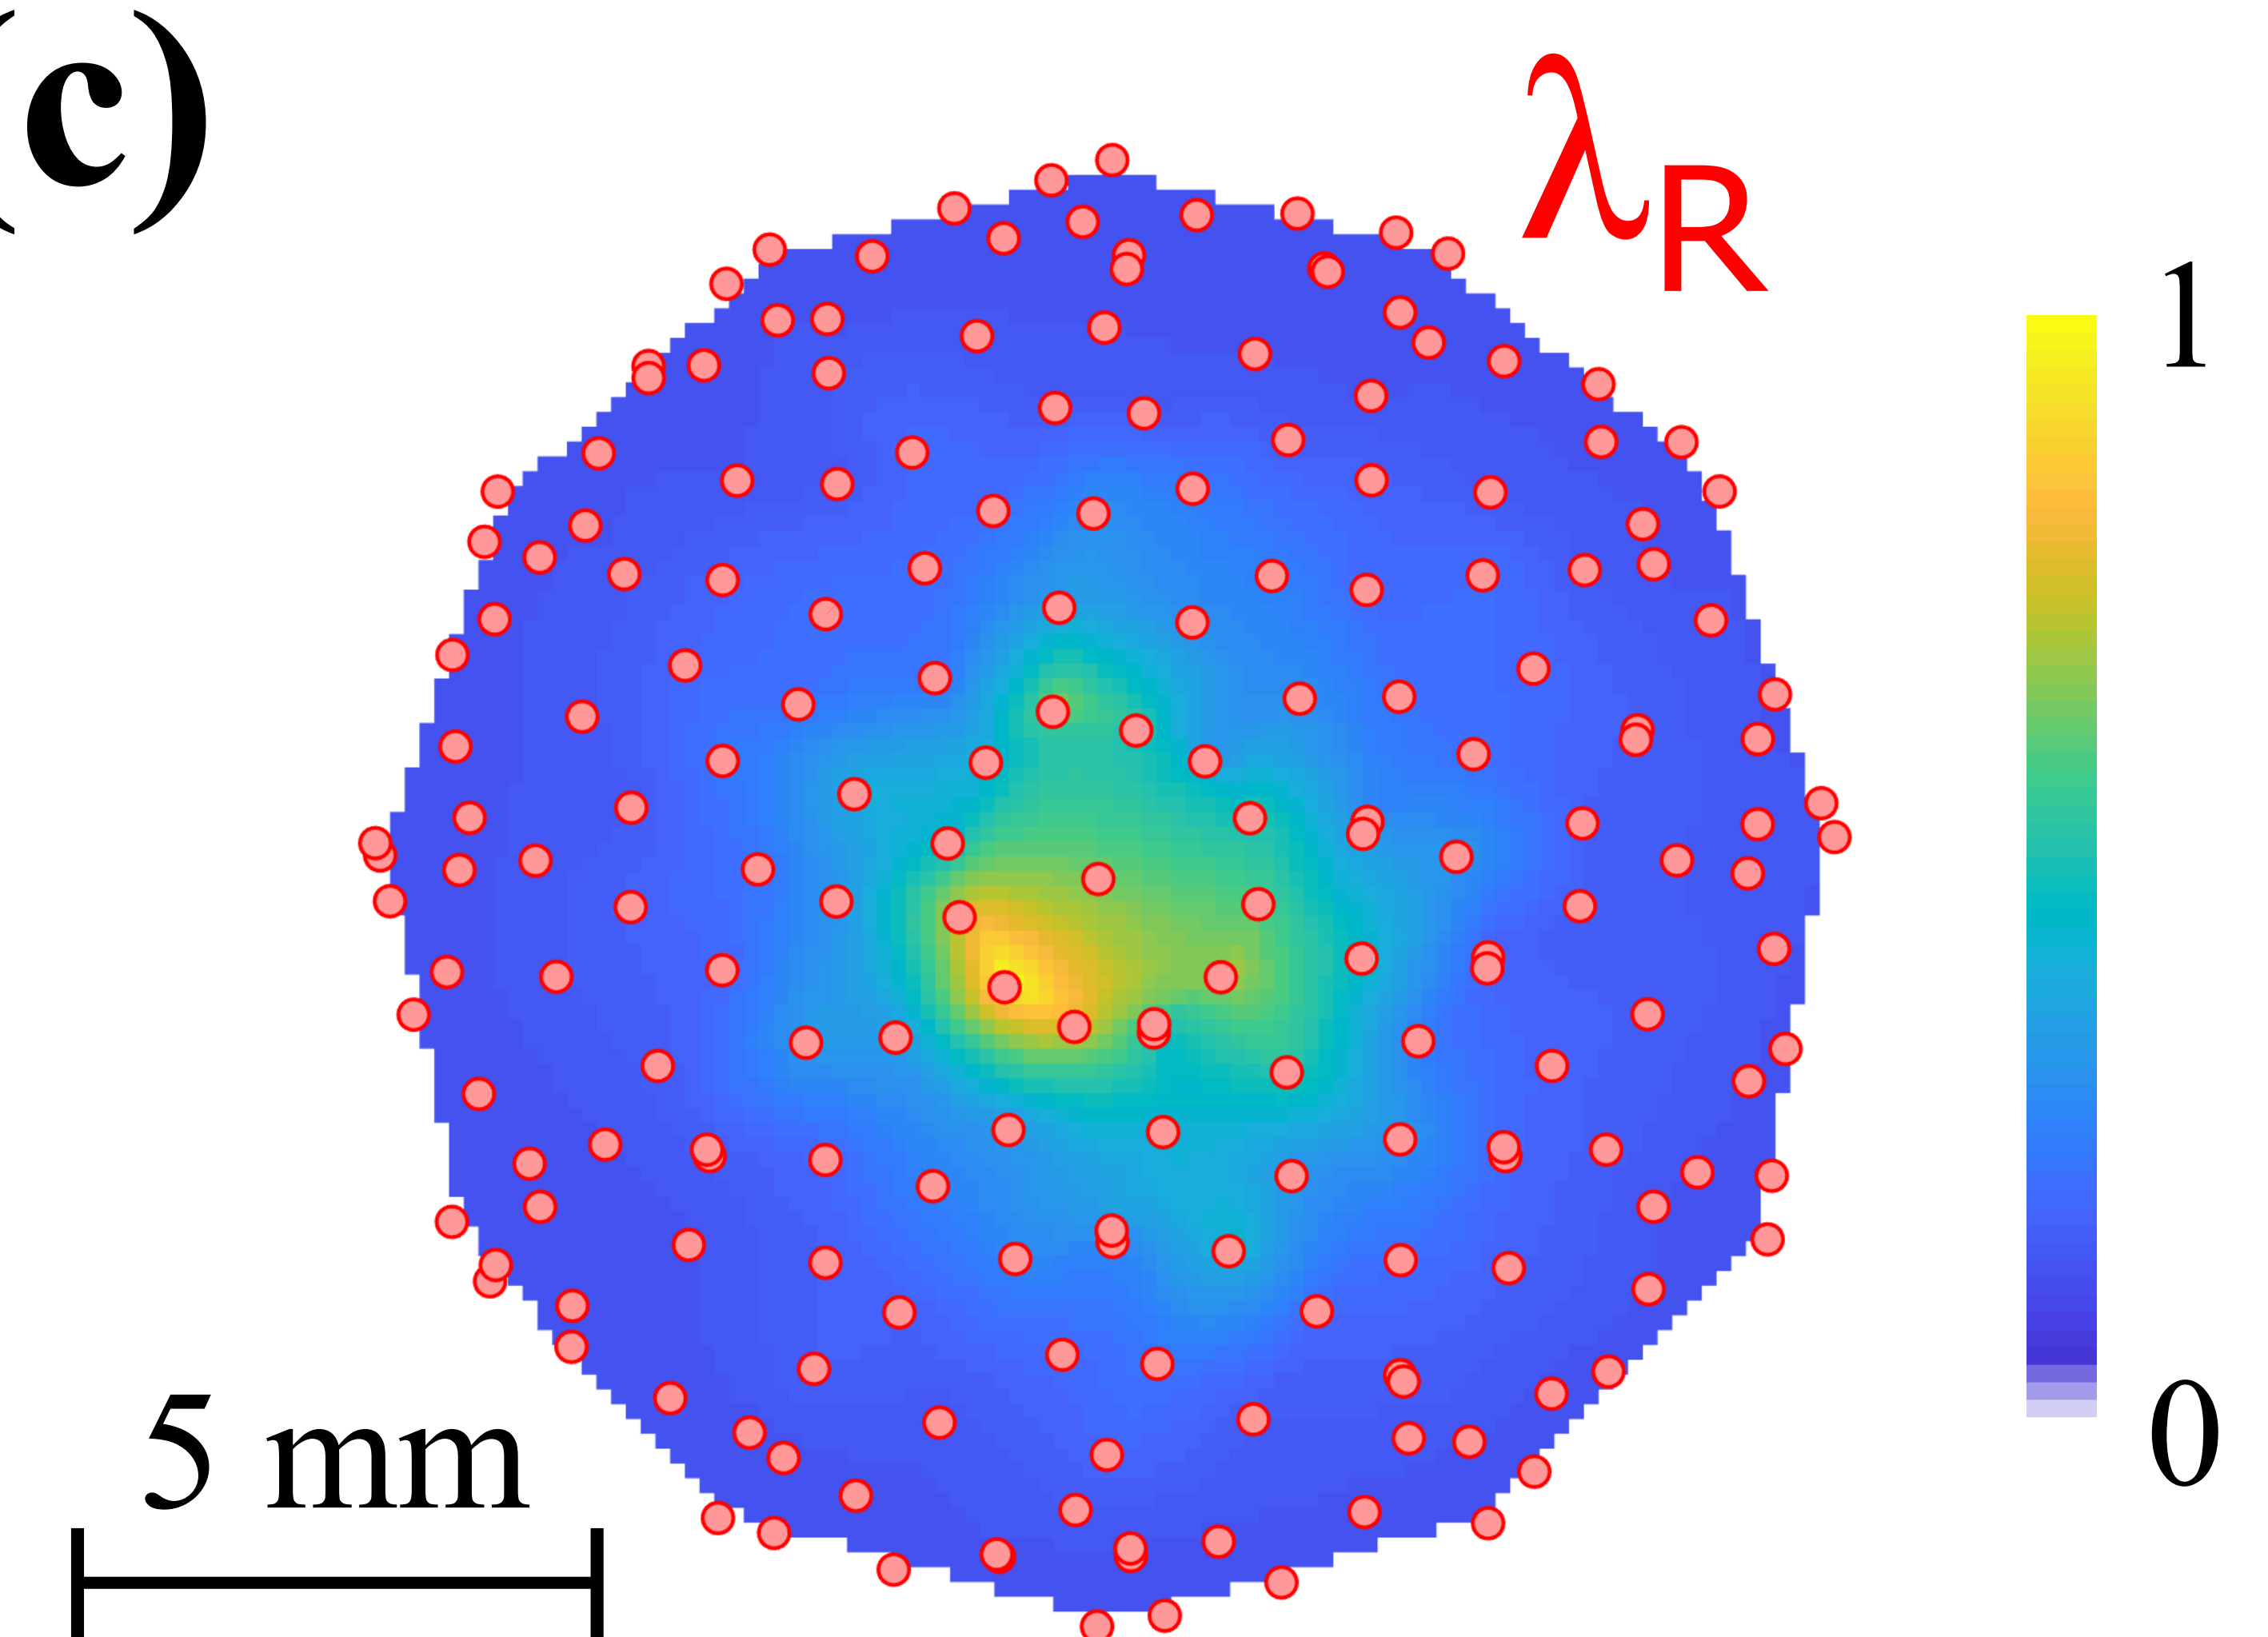**(d)**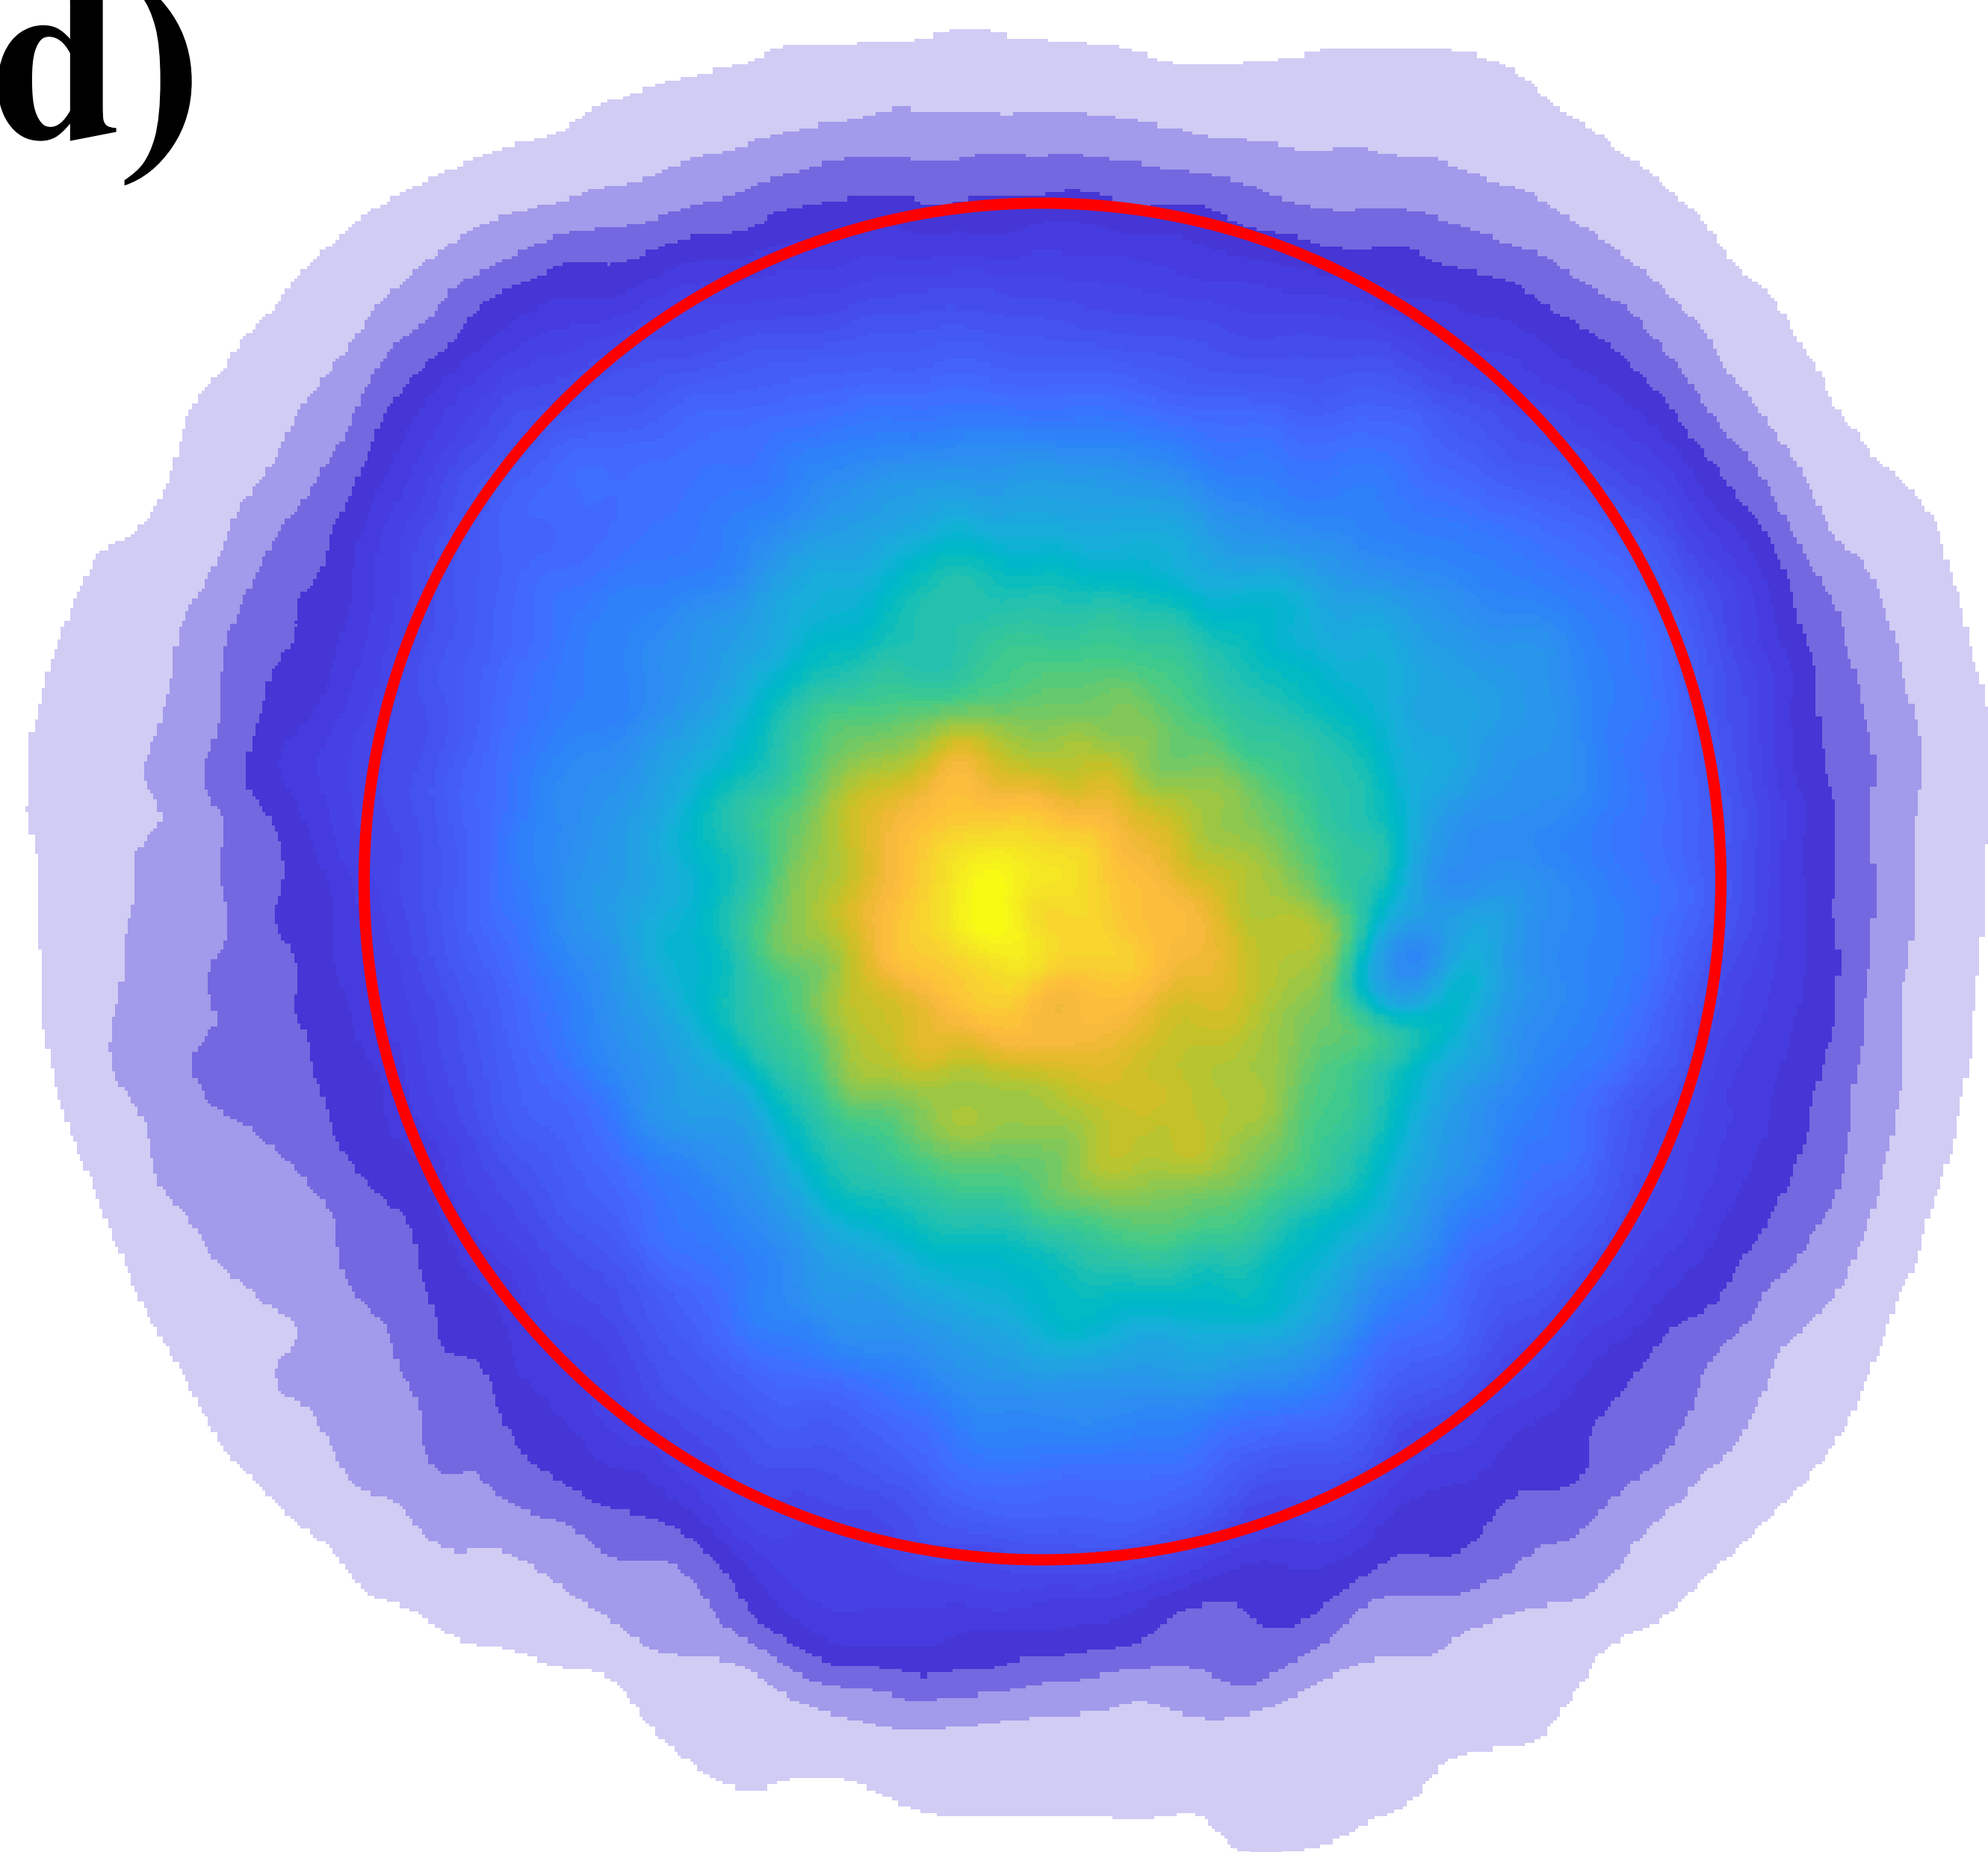**(e)**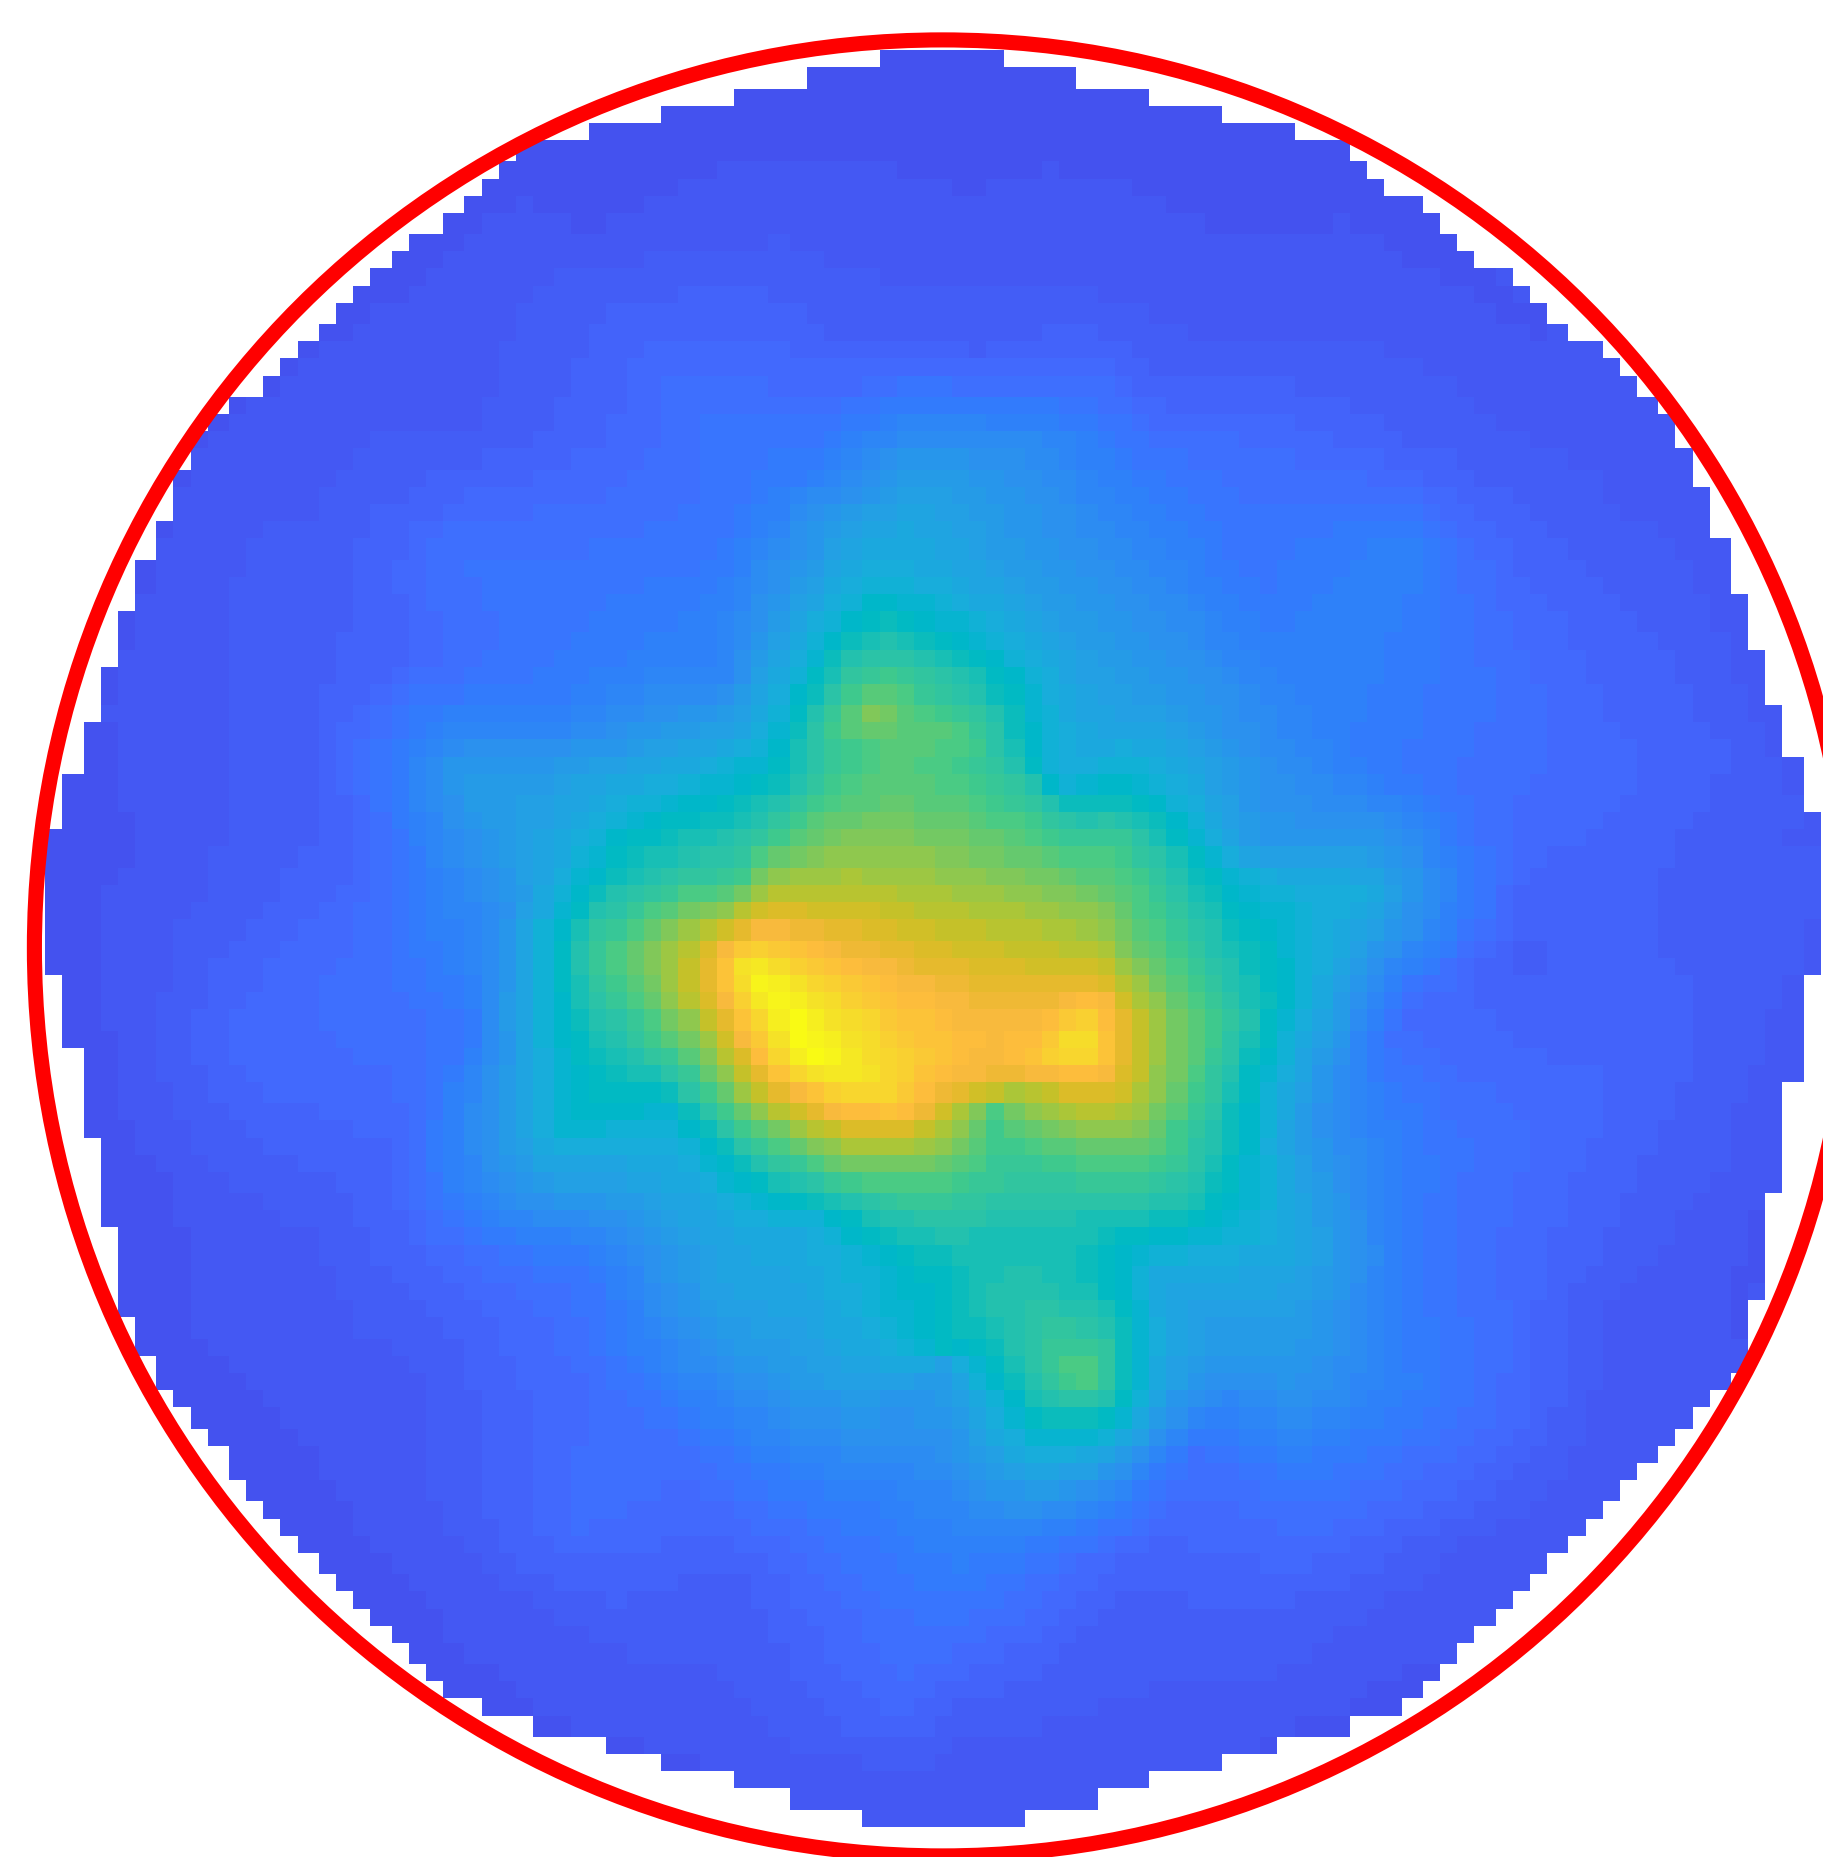**(f)**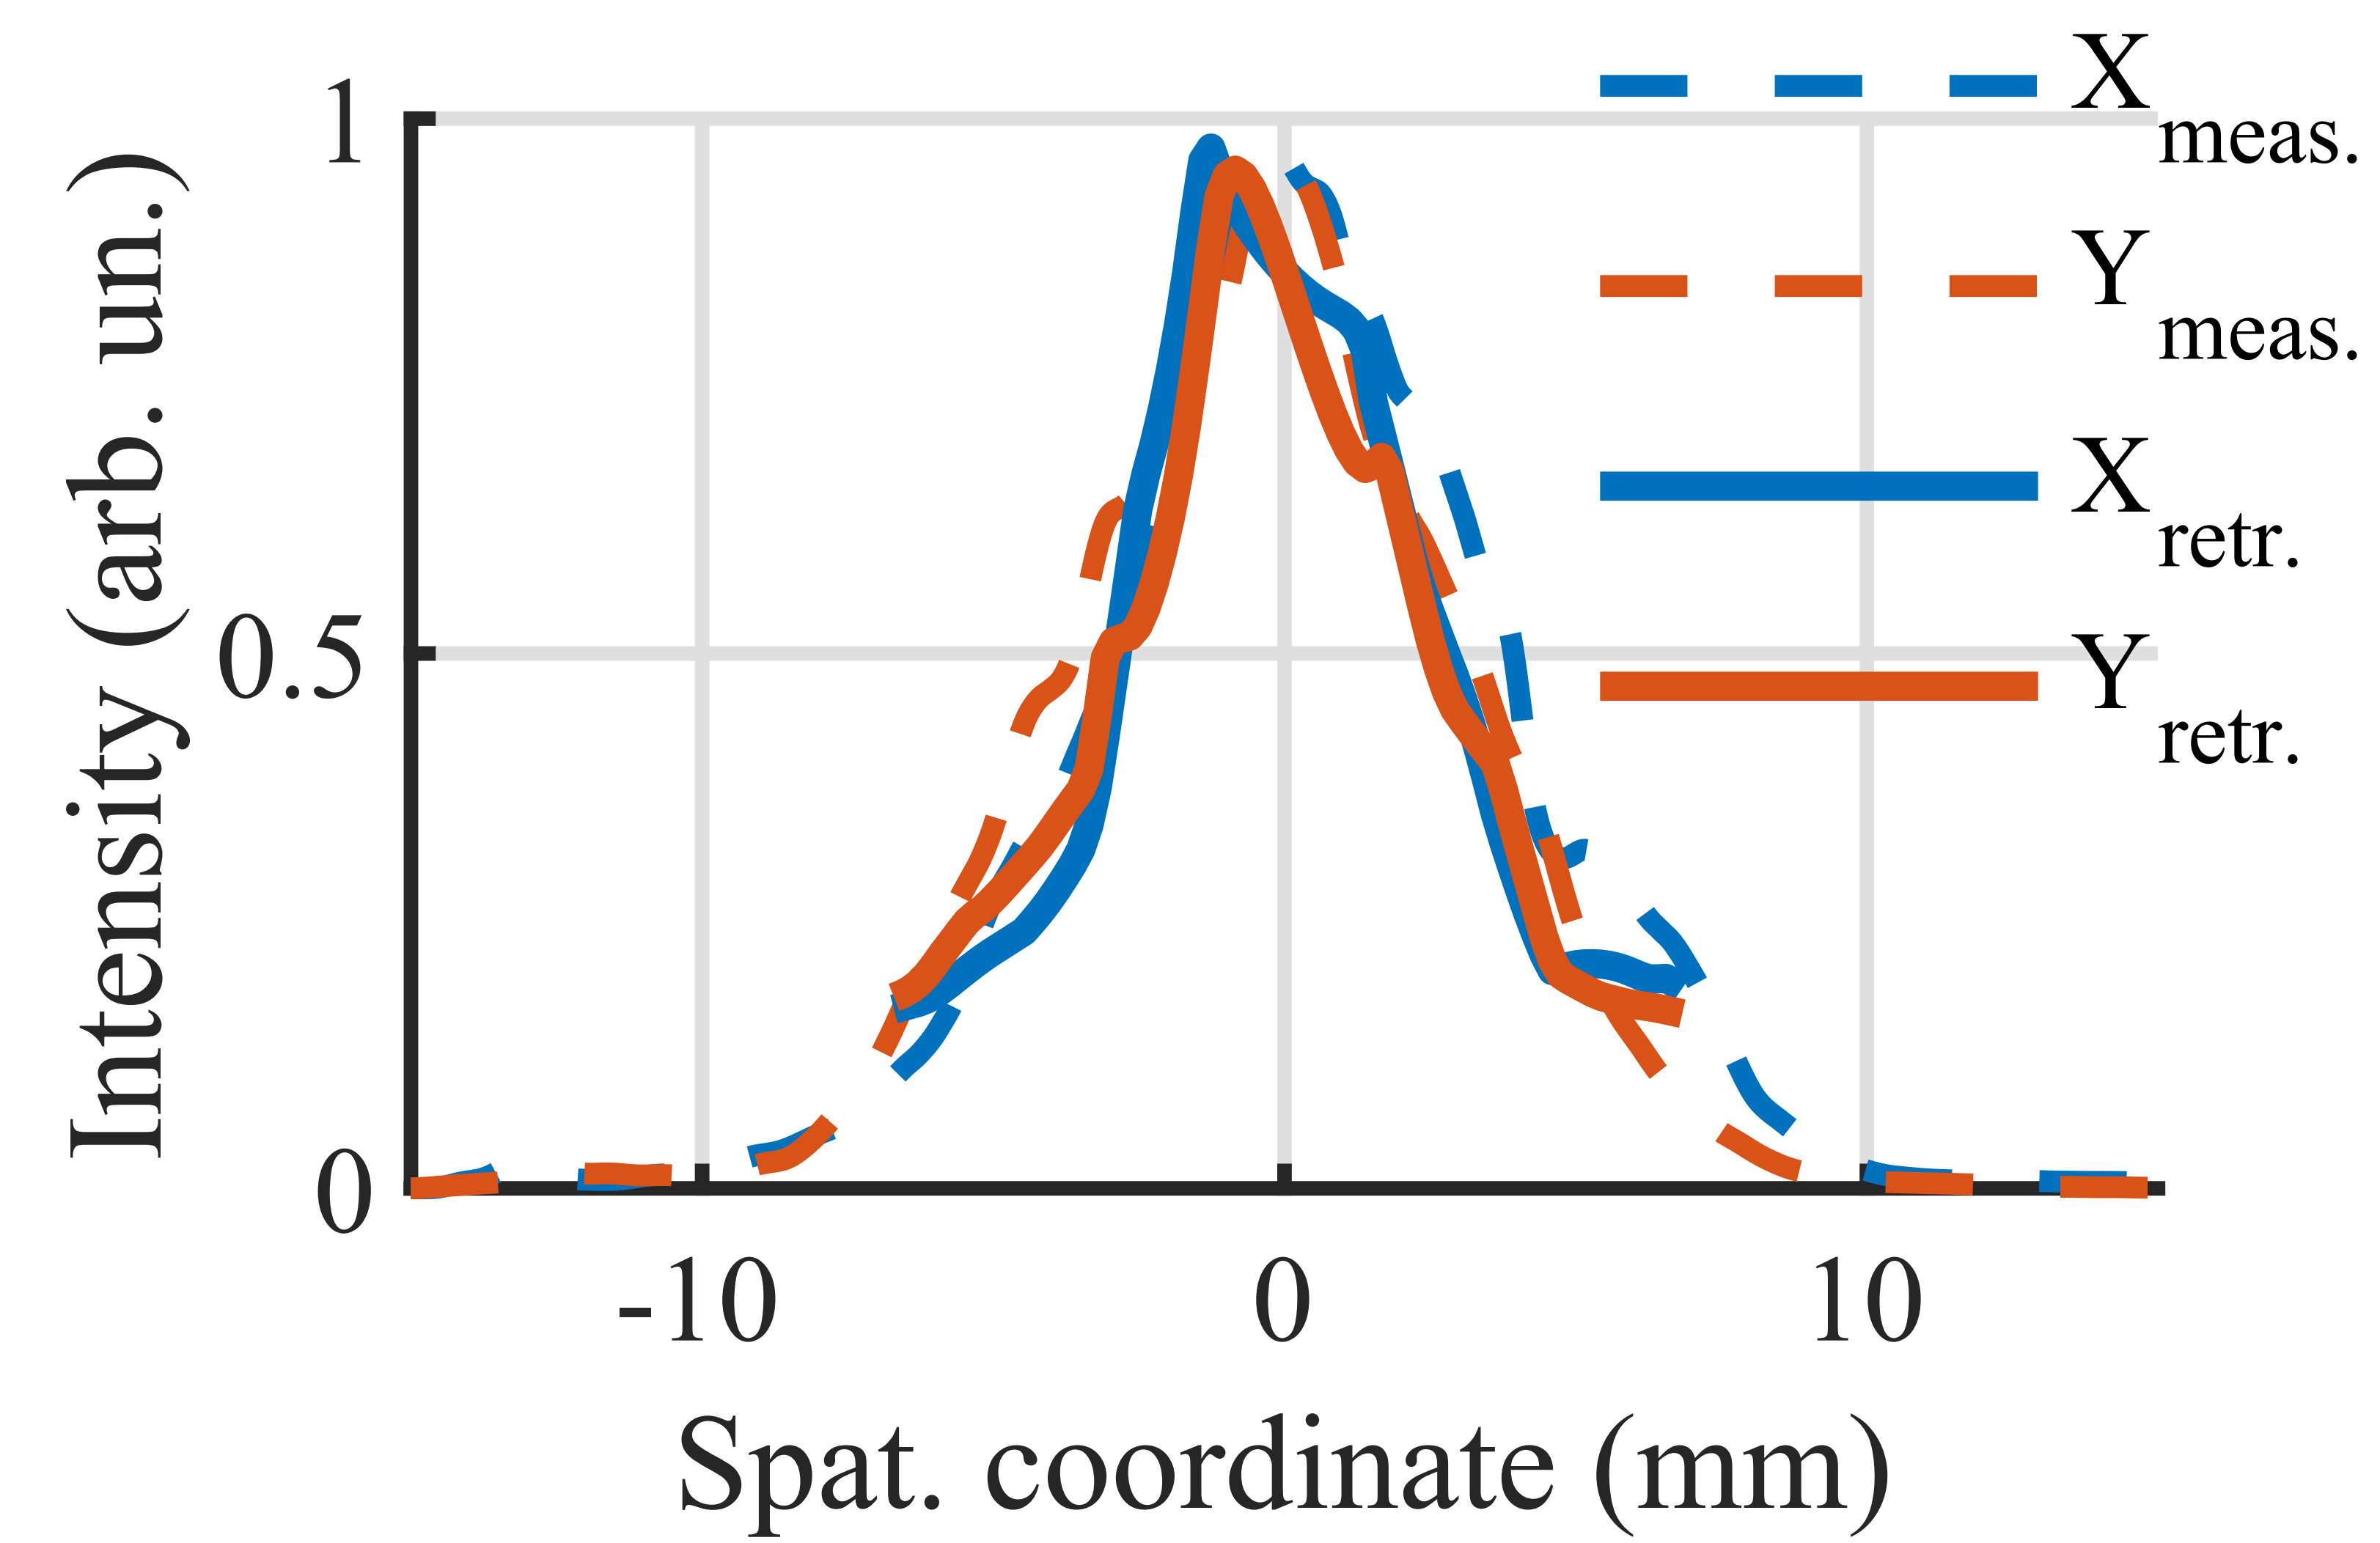

Supplement: Supplementary file 1 [file Rev2_IMPALA_NF_intensity.pdf]
